# Supplementary material for: Collecting and Analyzing Multidimensional Data with Local Differential Privacy
Source: arXiv:1907.00782 source file (2019-06-28)
Supplement: Supplementary file 1 [file appendix.tex]

\appendix

\begin{figure}[t]
\centering
\includegraphics[width=0.9\columnwidth]{multi-dim-pm-em-min.pdf}
 \caption{Plotting $\epsilon \{\WorstVar_P\big[t^{*}_i[A_j]\big]+1\}/d$ and $\epsilon \{\WorstVar_H\big[t^{*}_i[A_j]\big]+1\}/d$ with respect to $k/\epsilon$.}
 \label{multi-dim-pm-em-min}
\end{figure}

\begin{figure*}
  \centering
  \begin{tabular}{cccc}
  \multicolumn{4}{c}{}\\
    \hspace{2mm}\includegraphics[width=0.25\textwidth]{comparetruevalue0.pdf} &
    \hspace{-6mm}\includegraphics[width=0.25\textwidth]{comparetruevalue1over3.pdf} &
    \hspace{-6mm}\includegraphics[width=0.25\textwidth]{comparetruevalue2over3.pdf} &
    \hspace{-6mm}\includegraphics[width=0.25\textwidth]{comparetruevalue1.pdf}
    \\
    (a) $t_i = 0$ & (b) $t_i = \frac{1}{3}$ & (c) $t_i = \frac{2}{3}$ & (d) $t_i = 1$
   \end{tabular}
  \vspace{0pt}
  \caption{Noise variance for one-dimensional numeric data versus the privacy budget $\epsilon$.\vspace{-10pt}}
  \label{fig:variance} %% label for entire figure
\end{figure*}

{\color{blue}
\subsection{Noise variance of each mechanism for different input values.}

Fig.~\ref{fig:variance} reports each mechanism's noise variance for four different input values: $t_i = 0$, $t_i = \frac{1}{3}$, $t_i = \frac{2}{3}$, and $t_i = 1$. Observe that, in Fig.~\ref{fig:variance}(a)-(c), the proposed solutions PM and HM outperform Duchi et al.'s solution in almost all cases. Meanwhile, when $t_i = 1$, Duchi et al.'s solution slightly outperforms our solutions, since $t_i = 1$ is the best-case for the former but the worst-case for the latter. Hence, the proposed methods are a better choice overall.
%Taking into account all results in Fig.~\ref{fig:variance}, we believe that the overall performance of our solutions is superior to Duchi et al.'s method.

\subsection{Discussion of the value of $k$ in Eqn. \ref{eqn:multi-k}.}

The worst-case variance of $t^{*}_i[A_j]$ in Algorithm~4 with PM being used is computed by setting $t_i[A_j]$ as $\pm 1$ in $\Var_P\big[t^{*}_i[A_j]\big]$ of Lemma 6; i.e., the result denoted by $\WorstVar_P\big[t^{*}_i[A_j]\big]$ is given by
\begin{align}
 \frac{d(e^{\epsilon/(2k)}+3)}{3k(e^{\epsilon/(2k)} - 1)^2}   +  \left[ \frac{d\cdot e^{\epsilon/(2k)}}{k(e^{\epsilon/(2k)} - 1) } -1\right].
 \label{worst-case-variance-k-PM}
\end{align}

The worst-case variance of $t^{*}_i[A_j]$ in Algorithm~4 with HM being used is computed by setting $t_i[A_j]$ as $\pm 1$ in $\Var_H\big[t^{*}_i[A_j]\big]$ of Lemma 6; i.e., the result denoted by $\WorstVar_H\big[t^{*}_i[A_j]\big]$ is given by
\begin{align}
 \begin{cases}
\hspace{-1pt}\frac{d}{k} \hspace{-1pt} \left[ \frac{e^{\epsilon/(2k)}+3}{3e^{\epsilon/(2k)}(e^{\epsilon/(2k)}-1)} \hspace{-1pt}+ \hspace{-1pt}\frac{(e^{\epsilon/k}+1)^2}{e^{\epsilon/(2k)}(e^{\epsilon/k}-1)^2} \right] \hspace{-1pt}+\hspace{-1pt}  \left(\frac{d}{k}  \hspace{-1pt}-\hspace{-1pt} 1 \right )  , &  \hspace{-1pt}   \text{for }\epsilon/k > \epsilon^*,  \\ \hspace{-1pt}\frac{d}{k} \left(\frac{e^{\epsilon/k}+1}{e^{\epsilon/k}-1}\right)^2 +  \left(\frac{d}{k}  - 1 \right )  , &  \hspace{-1pt}  \text{for } \epsilon/k \leq \epsilon^*,
\end{cases}  \label{worst-case-variance-k-HM}
\end{align}

Given the expressions of $\WorstVar_P\big[t^{*}_i[A_j]\big]$ and $\WorstVar_H\big[t^{*}_i[A_j]\big]$ in the above Equations~(\ref{worst-case-variance-k-PM}) and (\ref{worst-case-variance-k-HM}),
we plot $\epsilon \{\WorstVar_P\big[t^{*}_i[A_j]\big]+1\}/d$ and $\epsilon\{\WorstVar_H\big[t^{*}_i[A_j]\big]+1\}/d$ with respect to $k/\epsilon$ in Fig.~\ref{multi-dim-pm-em-min}.
Obviously, it is observed that $\epsilon \{\WorstVar_P\big[t^{*}_i[A_j]\big]+1\}/d$ or $\epsilon\{\WorstVar_H\big[t^{*}_i[A_j]\big]+1\}/d$ is roughly minimized when $k/\epsilon = 0.4$, i.e., $k = \epsilon/2.5$.
So in order to minimize the worst-case variances $\WorstVar_P\big[t^{*}_i[A_j]\big]$ and $\WorstVar_P\big[t^{*}_i[A_j]\big]$ we specify $k$ by

$$k = \max\left\{1, \min\left\{d, \, \left\lfloor \frac{\epsilon}{2.5}\right\rfloor\right\}\right\}.$$

}
